# Supplementary material for: Clustering with Set Outliers and Applications in Relational Clustering
Source: arXiv:2509.16194 source file (2025-12-22)
Supplement: Supplementary file 1 [file appendix_old.tex]

\section{$k$-center clustering with tuple-outliers}
We start with a simpler geometric problem than the problem Definition~\ref{geomProb} that we call \loutlier. In this problem, we are given positive integers $k$ and $z$, a set $P$ of $n$ points in $\Re^2$ and a set $L$ of $m$ vertical lines with $m\ll n$ such that each point in $P$ lies on a line in $L$. Let $\ell(P)$ and $R(P)$ (for a subset $R\subseteq L$) are defined as in Section~\ref{sec:prelim}. 
The goal is to compute a set $P'\subseteq P$ with $|P'|=k$ and a set $L'\subseteq L$ with $|L'|=z$ such that $\rho(P',P\setminus L'(P))$ is minimized. 
s
Let $\rho^*_{k,z}(P,L)$ be the minimum possible value of the radius $\rho(P',P\setminus L'(P))$. We now provide a bicriteria approximation for the problem.
\todo{Vaishali: Add Blue Red Algorithm}
\begin{theorem}\todo{runtime}
    \label{thm:line-outlier}
    Given an instance $(P,L,k,z)$ of \loutlier, there exists an algorithm running in time $O(mk^3)$ that computes sets $P'\subseteq P$ and $L'\subseteq L$ such that $\rho(P',P\setminus L'(P))\leq 3\rho^*_{k,z}(P,L)$ and either (a) $|P'|\leq k(k+1)$ and $L'\leq z$ or (b) $|P|\leq k$ and $|L'|<z(z+1)$.
\end{theorem}

To provide the algorithm stated in Theorem~\ref{thm:line-outlier}, we first define a few terms. For a subset $X\subseteq P$, let $\Lambda(X)$ be the set of lines $\ell$ in $L$  that contain at least one point from $X$, i.e $|\ell(X)|>0$. Let $p\in P$, we say $p$ {\em $r$-covers} a point $q$ if $d(p,q)\leq r$. Further for a subset $X\subseteq P$ of points, let $cov(p,r,X)$ denote the set of points in $X$ that are $r$-covered by $p$. We then say point $p$ {\em $(r,X)$-hits} a line $\ell$ if $|cov(p,r,\ell(X))|>0$, that is there is a point in $\ell(X)$ that is $r$-covered by $p$.

We now provide an algorithm for \loutlier \ that takes a radius $r$ as input in addition to $(P,L,k,z)$. We can compute the optimum radius $\rho^*_{k,z}(P,L)$ using binary search. 

The algorithm is as follows:
\begin{enumerate}
    \item Initialize sets $L':=\emptyset$, $P':=\emptyset$, $U:=P$ \\ Interpret $L'$ as the set of outlier lines, $P'$ as the set of centers and $U$ as the set of uncovered points.
    % \item For each line $\ell\in L$:
    % \begin{itemize}
    %     \item Compute $\rho_k(\ell(P))$
    %     \item If $\rho_k(\ell(P))>r$, set $L'=L'\cup \ell$ and $U=P\setminus \ell(P)$. 
    %     \item If $|L'|>z$, Return {\sf NO}
    % \end{itemize}
    \item As long as there exists a point $p$ that $(r,U)$-hits more than $z$ lines:
    \begin{itemize}
        \item $P'=P'\cup p$
        \item $U = U\setminus cov(p,3r,U)$
        \item If $|P'|>k$, Return {\sf NO} 
    \end{itemize}
    \item If $|\Lambda(U)|< z(z+1)$ -- \#outlier lines is $\leq z^2$
    \begin{itemize}
        \item $L'=\Lambda(U)$
        \item Return $(P',L')$
    \end{itemize}
    \item Let $k' = k - |P'|$, for each line $\ell \in \Lambda(U)$:
    \begin{itemize}
        \item Compute $\rho_{k'}(\ell(U))$
        \item If $\rho_{k'}(\ell(U))>r$, set $L'=L'\cup \ell$ and $U=P\setminus \ell(U)$.   
        \item If $|L'|>z$, Return {\sf NO}
    \end{itemize}
    \item While $|U|>0$, let $u\in U$:
    \begin{itemize}
        \item Pick a point $u \in U$
        \item $P'=P'\cup p$
        \item $U = U\setminus cov(p,2r,U)$
        \item If $|P'|>k^2$, Return {\sf NO} 
    \end{itemize}
    \item Return $(P',L')$
\end{enumerate}

Next, we prove Theorem~\ref{thm:line-outlier} by showing that the above algorithm provides us the required guarantees.
\begin{proof}[Theorem~\ref{thm:line-outlier}]
%Since the optimal cost $\rho^*_{k,z}(P,L)$ must correspond to an inter-point distance, a $3$-approximation to the optimal cost can then be found by simulating a binary search on the list of all approximate interpoint distances.

Let $r=\rho(P^*,P\setminus L^*(P))$, we first show that running the algorithm with $(P,L,k,z)$ and $r$ returns sets $(P',L')$ satisfying the properties mentioned in the theorem statement. 
%
Note that $P'$ is the set of cluster center points and $L'$ is the set of outlier lines. 
%
Let $P' = \{p_1,p_2,\cdots,p_{|P'|}\}$ and $L'=\{\ell_i,\cdots,\ell_{|L'|}\}$ be the order in which the elements were added to the sets by the algorithm.
%
Further let $P^*$ and $L^*$ be a pair of optimal sets with $\rho(P^*,P\setminus L^*(P)) = \rho^*_{k,z}(P,L)$.

Let $x$ be the total number of points added to $P'$ in step (2). We now show that there are $x$ points $X=\{p^*_1,\cdots,p^*_x\}$ in $P^*$ that satisfies $cov(p^*_i,r,P) \subseteq cov(p_i,3r,P)$ for each $i\in [x]$. That is we show that each $p_i$ $3r$-covers all points that are $r$-covered by $p^*_i$ in the optimum solution. 

We will prove the claim by induction on $i\in [x]$. Suppose the claim is true $\forall j<i$. We now prove it for $i$.
Since point $p_i$ $(r,U)$-hits more than $z$ lines, there is an uncovered point $u\in U$ that does not lie on an outlier line in $L^*$. Thus $u$ is $r$-covered by $p$ and also $r$-covered by some $p^*_i\in P^*$. Note that $\forall j<i$, $p^*_i\neq p^*_j$ -- if not $u$ must have been $3r$-covered by some $p_j$ and thus $u\notin U$. Since the ball of radius $r$ around $p_i^*$ and $p_i$ intersect, $p_i$ $3r$-covers all points that are $r$-covered by $p^*_i$ and so $cov(p^*_i,r,P) \subseteq cov(p_i,3r,P)$.
%%%%%%%%

Note that at the end of step (2), $|P'|\leq k$. Consider $U_2$ to be the set $U$ of uncovered points after step (2). Each uncovered point in $U_2$ either lies on an outlier line in $L^*$ or is covered by a center $p^*\in P^*\setminus X$ that $(r,U_2)$-hits at most $z$ lines. Thus $|\Lambda(U)|<z+z.k=z(k+1)$.
%
If $k\leq z$, then $|\Lambda(U)|<z(z+1)$ and the algorithm in step (3) returns $(P',L')$ such that $\rho(P',P\setminus L'(P))\leq 3\rho^*_{k,z}(P,L)$ and $|P|\leq k$ and $|L'|< z(z+1)$ proving the Theorem.
%%%%%%%%%%

We are now left to prove the Theorem when $k>z$. Recall that $k'=k-|X|$. Step (4) identifies obvious outlier lines in $L^*$, those that need more than $k'$ centers and includes them in $L'$. Observe that no point in $U_2$ is $r$-covered by any point in $X$ and thus if a point in $U_2$ is $r$-covered in the solution, it is covered by some point in $P^*\setminus X$. If for a line $\ell$, $\rho_{k'}(\ell(U))>r$, then points in $\ell(U)$ cannot be $r$-covered by a set of $k'$-points in $P^*\setminus X$ and so $\ell$ must be an outlier. Thus every line $\ell$ added to $L'$ in step (4) must be an outlier in $L^*$ as well. 

At the end of step (4), every line $\ell\in L\setminus L'$ has $\rho_{k'}(\ell(U))\leq r$, thus $k'$ centers are enough to $r$-cover all the point in $\ell(U)$. 

At this point, all uncovered points can be $r$-covered using at most $k'+k'.z$ centers. Step (5) performs a greedy $2$-approximation to cover all point in $U$. This yields at most $k'+k'.z$ centers that $2r$-cover all points in $U$.

Since $k>z$, $|P'|\leq (k-k')+k'+k'.z \leq k+k^2 = k(k+1)$. Thus step (5) returns $(P',L')$ such that $\rho(P',P\setminus L'(P))\leq 3\rho^*_{k,z}(P,L)$ and $|P|\leq k(k+1)$ and $|L'|\leq z$.

Thus we have shown that when $r=\rho(P^*,P\setminus L^*(P))$, the algorithm returns sets $(P',L')$ with the required guarantees. It is also easy to observe that if the algorithm for a given radius $r'$ returns sets $(P',L')$ then $P'$ $3r'$-covers all points in $P\setminus L'(P)$ since at the end of the algorithm the set of uncovered points $U=\emptyset$.

Finally to find $\rho(P^*,P\setminus L^*(P))$, we do a binary search over all possible distances and run the algorithm during each step.
%%%%%%%%%
\end{proof}
